# Supplementary material for: A Stable and Efficient Covariate-Balancing Estimator for Causal Survival Effects
Source: arXiv:2310.02278 source file (2024-05-15)
Supplement: Supplementary file 1 [file proof-scratch.tex]

is suffices to 
suffices to show that the variance of 
it suffices to show that 

$\hat\phi$ and $\phi$ have mean zero,

\quad \text{ for } \quad \phi_i = \hat S_t(a,X_i) - \E \hat S_t(a,X_i) + \gamma_u(Z_i) \{ 1(E_i, \tilde T_i=u) - \lambda_u(Z_i) \} \]
Thus, it 

which we apply seperately for each $u \in 1 \ldots t$.

applied separately for each $u$

to 
\ref{lemma:This is implied by the fourth-root rate of convergence
\item 

approximation to $\psi(\lambda)$

$\psi

first term in this decomposition is $\psi_n(\lambda)-\psi(\lambda) + o_p(n^{-1/2})$, 
which is simply different notation for the first term $\frac{1}{n} \sum_{i=1}^n S_t(a,X) - \E S_t(a, X)$ in the average of the influence function $\phi$ in \eqref{eq:claim-appendix}. To see this, observe that the 
difference $\{ \psi_n(\hat\lambda)-\psi(\hat\lambda)\} - \{ \psi_n(\lambda)-\psi(\lambda)\}$ 
is an average of independent and identically distributed mean-zero terms with variance tending to zero as $\hat\lambda \to \lambda$.
\item The second term in this decomposition is ...
\item The third term in this decomposition, the remainder ..., is 
\end{enumerate}

$\hat \lambda \to \lambda$,
so $\hat S \to S$

\item The second term in this decomposition is

In this decomposition, $\psi_n(\lambda)

$\psi_n(\lambda)$ is the average of $n$ independent and identically distributed terms
$S_i = \prod_{u \le t}\left( 1- \lambda_u(a,Z_i) \right)$ and $\psi

The first term is simply the difference between an average of independent identically distributed terms and  
in this decomp
Here by averaged EIF I mean with $S=\hat S$; it takes another step to show that's negligibly different from its value with $S=S$.
\[ P_n i_{\hat \lambda} - i_{\lambda}  = o(n^{-1/2})  \ \text{ because } \  \hat \lambda \to \lambda \implies i_{\hat \lambda} \to i_{\lambda} \]
so this difference is an average of independent mean zero things converging to zero, i.e., it's $o(n^{-1/2})$ by Chebyshev's inequality.

\begin{enumerate}
\item Explain how we break down the estimation of $\psi(t,a)$ into $t$ different estimation problems. Show an error decomposition or something motivating this.
\item Do an error decomposition for those estimation problems involving an imbalance term, the term dependent on rates for S, influence function terms, and whatever else
\item Show that everything but the influence function terms is negligible
\end{enumerate}

In this section, we prove our main theoretical result. We first adapt a result from \citep{hirshberg2021augmented}. Our insight is that we can treat our balancing weight estimator of $\psi(t,a)$ as $|t|$ independent estimators, each of which is estimating a \textit{weighted} average of the conditional hazard at time $u \le t$. We formally define one such estimation problem and the associated augmented minimax linear estimator (AMLE) below.

Fix a time $u \in \mc T$, a treatment $a \in \{0, 1\}$ and a function $g(x): \mc X \rightarrow (0, 1)$. Define an additional indicator random variable $V = \one(\td T \ge u)$. Suppose we observe $n$ observations $(Y_i, Z_i)_{i=1}^n$, where $Y_i = g(X_i)\one(\td T_i=u, E_i=1)$ and $Z_i = (V_i, A_i, X_i)$. We  want to estimate $$\theta(m_0) = \E[h((V_i, A_i, X_i); m_0)],$$ where:
$$m_0(v,a_0,x) = \E[Y | V=v, \one(A=a)=a_0, X=x]$$
and 
$$h((v, a_0, x); m) = m(1, 1, x).$$ Then the augmented minimax linear estimator of $\psi(m_0)$ is:
$$
\hat \theta = \frac{1}{n}\sum_{i=1}^n \left\{ h(Z_i; \hat m) + \hat \gamma_i (Y_i - \hat m(Z_i)) \right\}
$$
where $\hat m$ is an estimator of $m_0$, and $\hat \gamma$ is defined as:
\begin{align*}
\hat \gamma &= \arg \min_{\gamma \in \R^n} I^2(\gamma) + \frac{\sigma^2}{n^2}\norm{\gamma}^2_2\\
I(\gamma) &= \sup_{f \in \mc F} P_n[\gamma_i f(Z_i) - f(Z_i)]
\end{align*}

The following lemma is a straight-forward adaptation of Theorem 1 from \citep{hirshberg2017augmented}:
\begin{lemma}
\label{lem:amle}
Assume that $\mc F$ is uniformly bounded and pointwise closed; $\mc F$, $\gamma \mc F$ and $h(\cdot, \mc F)$ are Donsker; and $h(Z,\cdot)$ is pointwise bounded and mean-square equicontinuous on $\mc F$ in the sense that $\sup_{f \in \mc F}|h(z, f)| < \infty$ for each $z \in \mc Z$ and $\lim_{r \rightarrow 0}\sup _{f \in \mc F_r}\norm{h(\cdot, \mc F)}_{L_2(P)} = 0$. Further assume that $\hat m$ has the tightness and consistency property that:
\begin{align*}
&\norm{\hat m - m_0} = O_p(1)\\
&\norm{\hat m - m_0}_{L_2(P_n)} = o_p(1)
\end{align*}
Under these conditions, we have that:
$$
\hat \theta - P_n[h(Z_i;m_0) - \gamma_0(Z_i)(m(Z_i) - Y_i)] = o_p(n^{-1/2})
$$
where $\gamma_0(Z_i)$ is the limit of $\hat \gamma_i$ i.e.,
$$
\frac{1}{n}(\hat\gamma_i - \gamma_0(Z_i)) \rightarrow_P 0.
$$
\end{lemma}

% \paragraph{Application to the proof}
% Set $g(x) = \frac{\hat S(t|a,X) \hat S(u-|a,X)}{\hat S(u|a,X)}$, where $\hat S$ has been estimated from an auxiliary sample, so is an indepedent function, and is also in $(0, 1)$. $h$ and $m$ in our proof will be similar to this problem. Concretely, $m$ is:
% \begin{align*}
% m(v,a_0,x) &= \E[g(X)\one(\td T=u,E=1)|\one(\td T\ge u)=v, \one(A=a)=a_0, X=x]\\
% m(1,1,x) &= \E[g(X)\one(\td T=u,E=1)|\td T\ge u, A=a, X=x]\\
% &= g(x)\lambda(u|a,x)
% \end{align*}
% (here $g(x)$ does not depend on $u$ or $a$ anymore). The AMLE estimator of $\theta$ is:
% \begin{align*}
% &P_n \left[g(X_i)\hat\lambda(u|a,X_i)\right]\\
% &+P_n\left[\one(\td T_i\ge u,A_i=a)\hat\omega_u(X_i) g(X_i)(\one(\td T_i\ge u, E_i=1) - \hat \lambda(u|a,X_i))\right]
% \end{align*}
% and the influence function sample average is:
% \begin{align*}
% &P_n \left[g(X_i)\lambda_0(u|a,X_i)\right]\\
% &+P_n\left[\one(\td T_i\ge u,A_i=a)\omega_{u,0}(X_i) g(X_i)(\one(\td T_i\ge u, E_i=1) - \lambda_0(u|a,X_i))\right]
% \end{align*}

Non-Linear AMLE
\[ f(\lambda) = f(\hat\lambda) + f'(\hat\lambda)(\lambda-\hat\lambda) + rem
\quad \text{ where } \quad f'(\hat\lambda)(\lambda-\hat\lambda) = P_n \hat\gamma (\lambda-\hat\lambda) \]

Our estimation of $\one(\td T \ge u, A=a)\omega_u$ is exactly estimation of $\gamma$.

where 
$$\hat \omega_u = \arg \min_{\omega_u \in \R^n} I^2(\omega_u) + \frac{\sigma^2}{n^2}\norm{\omega_u}^2_2
$$ and
$$
I(\omega_u) = \sup_{f \in \mc F} P_n[\one(\td T_i \ge u, A_i=a)\omega_u(X_i)f(X_i) - f(X_i)]
$$
therefore we can use the bound in lemma \ref{lem:amle}.

We additionally prove the following useful lemmas:

%\begin{lemma}
%\label{lem:rate_S}
%$$
%\norm{\hat S_t(a,X) - S_t(a,X)}_{L_2(P_n)} = O\left(\norm{\hat \lambda_u(a,X) - \lambda_u(a,X)}_{L_2(P_n)}\right)
%$$ for each $a \in \{0, 1\}$ and $t \in \mc T$
%\end{lemma}
%\begin{proof}
%\begin{align*}
%\norm{\hat S(t|a,X) - S_0(t|a,X)}_{L_2(P_0)} &= \norm{\sum_{u \le t} \hat S(t|a,X)\frac{S^0(u-|a,X)}{\hat S(u|a,X)}\left(\lambda_0(u|a,X) - \hat \lambda(u|a,X)\right)}_{L_2(P_0)} \quad \text{lemma \ref{lem:decompose_S}}\\
%&\le |\mc T|\max_{u \le t}\norm{\hat S(t|a,X)\frac{S^0(u-|a,X)}{\hat S(u|a,X)}\left(\lambda_0(u|a,X) - \hat \lambda(u|a,X)\right)}_{L_2(P_0)}\\
%&\le |\mc T|\max_{u \le t}\norm{\lambda_0(u|a,X) - \hat\lambda(u|a,X)}_{L_2(P_0)}
%= o_p(n^{-1/4}),
%\end{align*}
%since $\hat S(t|a,X) \le \hat S(u|a,X)$ for $u \le t$ and $S(u|a,X) \le 1$ for $u \in \mc T$
%\end{proof}

% \begin{lemma}
% \begin{align*}
% \phi(t,a,\hat\lambda,\hat\omega) - \phi(t,a,\lambda_0,\omega_0) = 
% \end{align*}
% \end{lemma}
% \begin{proof}
% \begin{align*}
% \phi(t,a,\hat\lambda,\hat\omega) - \phi(t,a,\lambda_0,\omega_0) = 
% \end{align*}
% \end{proof}

% Recall that the influence function parameterized by $\eta = (\lambda, \omega)$ is $\varphi(t,a,\lambda,\omega) = \phi(t,a,\lambda,\omega) - \psi(t,a)$, where:
% \begin{align*}
% &\phi(t, a, \lambda, \omega)(O) = S(t|a,X)\\
% &- \sum_{u\le t}S(t|a,X)\frac{S(u-|a,X)}{S(u|a,X)}\one(\td T \ge u,A=a)\omega(u|a,X)\left(\one(\td T=u,E=1)- \lambda(u|a,X)\right)
% \end{align*}
% Denote $\hat\psi$ and $\psi_0$ for the estimator and the ground truth estimand.

\begin{proof}[Proof of theorem \ref{thm:efficiency}] We begin by decomposing the error:
\begin{align*}
\hat \psi(t, a) - \psi_0(t, a) &= P_n[\phi(t,a,\lambda_0,\omega_0)(O_i)] - \psi(t,a) + \hat \psi(t, a) - P_n[\phi(t,a,\lambda_0,\omega_0)(O_i)]\\
&= P_n[\varphi(t,a,\lambda_0,\omega_0)(O_i)] + \hat \psi(t, a) - P_n[\phi(t, a, \lambda_0, \omega_0)(O_i)]
\end{align*}
We need to show that
\begin{align*}
\hat \psi(t, a) - P_n[\phi(t, a, \lambda_0, \omega_0)(O_i)] &= P_n[\phi(t,a,\hat\lambda,\hat\omega)(O_i) - \phi(t,a,\lambda_0,\omega_0)(O_i)]\\
&= o_p(n^{-1/2})
\end{align*}
We will break this error into $t$ terms. First, we 
\begin{align*}
&P_n[\phi(t,a,\hat\lambda,\hat\omega)(O_i) - \phi(t,a,\lambda_0,\omega_0)(O_i)]\\ 
&= P_n^k[\hat S_{-k}(t|a,X_i) - S_0(t|a,X_i)]\\
&-\sum_{u\le t}P_n^k\left[\one(\td T_i\ge u,A_i=a)\hat\omega_u(X_i)\hat S_{-k}(t|a,X_i)\frac{\hat S_{-k}(u-|a,X_i)}{\hat S_{-k}(u|a,X_i)}(\one(\td T_i\ge u, A_i=a) - \hat \lambda_{-k}(u|a,X_i))\right]\\
&+\sum_{u\le t} P_n^k\left[\one(\td T_i\ge u,A_i=a)\omega_{u,0}(X_i) S_0(t|a,X_i)\frac{S_0(u-|a,X_i)}{S_0(u|a,X_i)}(\one(\td T_i\ge u, A_i=a) - \lambda_0(u|a,X_i))\right]\\
&= \sum_{u\le t}\hat S_{-k}(t|a,X_i)\frac{S_0(u-|a,X_i)}{\hat S_{-k}(u-|a,X_i)}\frac{\hat S_{-k}(u-|a,X_i)}{\hat S_{-k}(u|a,X_i)}(\lambda_0(u|a,X_i) - \hat\lambda_{-k}(u|a,X_i)) \quad (\text{lemma})\\
&-\sum_{u\le t}P_n^k\left[\one(\td T_i\ge u,A_i=a)\hat\omega_u(X_i)\hat S_{-k}(t|a,X_i)\frac{\hat S_{-k}(u-|a,X_i)}{\hat S_{-k}(u|a,X_i)}(\one(\td T_i\ge u, A_i=a) - \hat \lambda_{-k}(u|a,X_i))\right]\\
&+\sum_{u\le t}P_n^k\left[\one(\td T_i\ge u,A_i=a)\omega_{u,0}(X_i) S_0(t|a,X_i)\frac{S_0(u-|a,X_i)}{S_0(u|a,X_i)}(\one(\td T_i\ge u, A_i=a) - \lambda_0(u|a,X_i))\right]\\
&= \sum_{u\le t} (R_{1,u} - R_{2,u} + R_{3,u})
\end{align*}
where:
\begin{align*}
R_1 &= P_n^k\left[\hat S_{-k}(t|a,X_i)\frac{\hat S_{-k}(u-|a,X_i)}{\hat S_{-k}(u|a,X_i)}\left(\frac{S_{0}(u-|a,X_i)}{\hat S_{-k}(u-|a,X_i)}-1\right)(\lambda_0(u|a,X_i) - \hat\lambda_{-k}(u|a,X_i))\right]\\
R_2 &= P_n^k \left[\hat S_{-k}(t|a,X_i)\frac{\hat S_{-k}(u-|a,X_i)}{\hat S_{-k}(u|a,X_i)}\hat\lambda_{-k}(u|a,X_i)\right]\\
&+P_n^k\left[\one(\td T_i\ge u,A_i=a)\hat\omega_u(X_i) \hat S_{-k}(t|a,X_i)\frac{\hat S_{-k}(u-|a,X_i)}{\hat S_{-k}(u|a,X_i)}(\one(\td T_i\ge u, A_i=a) - \hat \lambda_{-k}(u|a,X_i))\right]\\
&- P_n^k \left[\hat S_{-k}(t|a,X_i)\frac{\hat S_{-k}(u-|a,X_i)}{\hat S_{-k}(u|a,X_i)}\lambda_0(u|a,X_i)\right]\\
&-P_n^k\left[\one(\td T_i\ge u,A_i=a)\omega_{u,0}(X_i)\hat S_{-k}(t|a,X_i)\frac{\hat S_{-k}(u-|a,X_i)}{\hat S_{-k}(u|a,X_i)}(\one(\td T_i\ge u, A_i=a) - \lambda_0(u|a,X_i))\right]\\
R_3 &= P_n^k\Bigg[\one(\td T_i\ge u,A_i=a)\omega_{u,0}(X_i)\left(S_0(t|a,X_i)\frac{S_0(u-|a,X_i)}{S_0(u|a,X_i)} - \hat S_{-k}(t|a,X_i)\frac{\hat S_{-k}(u-|a,X_i)}{\hat S_{-k}(u|a,X_i)}\right)\\
&\quad\quad\quad\times(\one(\td T_i\ge u, A_i=a) - \lambda_{0}(u|a,X_i))\Bigg]
\end{align*} 
\khiem{@David could you help me correct this?} We proceed to bound terms $R_{3,u}, R_{2,u}, R_{1,u}$ in that order. Note that $R_{3,u}$ is a sum of \textit{independent} mean-0 and random variables, each of which is also converging to $0$ since $\hat S_{-k}$ is consistent, therefore $R_3 = o_p(n^{-1/2})$. The random variables are independent due to $S_{-k}$ being trained on $I_{-k}$. To bound term 2, we reduce it to the estimation problem previously mentioned, by setting $g(x) = \hat S_{-k}(t|a,x)\frac{\hat S_{-k}(u-|a,x)}{\hat S_{-k}(u|a,x)}$, therefore by lemma~\ref{lem:amle} term $R_2$ is also $o_p(n^{-1/2})$ by our assumptions. To bound term $R_1$, we use a standard argument from double machine learning \citep{chernozhukov2018double} concerning empirical process and cross-fitting. Specifically write $R_1$ as:
\begin{align*}
R_1 &= (P_n^k - P_0)\left[\hat S_{-k}(t|a,X_i)\frac{\hat S_{-k}(u-|a,X_i)}{\hat S_{-k}(u|a,X_i)}\left(\frac{S_{0}(u-|a,X_i)}{\hat S_{-k}(u-|a,X_i)}-1\right)(\lambda_0(u|a,X_i) - \hat\lambda_{-k}(u|a,X_i))\right]\\
&+ P_0\left[\hat S_{-k}(t|a,X_i)\frac{\hat S_{-k}(u-|a,X_i)}{\hat S_{-k}(u|a,X_i)}\left(\frac{S_{0}(u-|a,X_i)}{\hat S_{-k}(u-|a,X_i)}-1\right)(\lambda_0(u|a,X_i) - \hat\lambda_{-k}(u|a,X_i))\right]\\
\end{align*}
Conditional on $I_{-k}$, the first term has mean zero and variance bounded by:
\begin{align*}
&\var\left[ \hat S_{-k}(t|a,X_i)\frac{\hat S_{-k}(u-|a,X_i)}{\hat S_{-k}(u|a,X_i)}\left(\frac{S_{0}(u-|a,X_i)}{\hat S_{-k}(u-|a,X_i)}-1\right)(\lambda_0(u|a,X_i) - \hat\lambda_{-k}(u|a,X_i)) \Bigg\vert I_{-k}\right]\\
&\le \frac{K}{n}\norm{\left(\frac{\hat S_{0}(u-|a,X_i)}{\hat S_{-k}(u-|a,X_i)}-1\right)(\lambda_0(u|a,X_i) - \hat\lambda_{-k}(u|a,X_i))}_{L_2(P_0)}^2 = o_p(n^{-1})
\end{align*}
% \begin{align*}
% \E\left[(P_n^k - P_0)\left[\hat S_{-k}(t|a,X_i)\frac{\hat S_{-k}(u-|a,X_i)}{\hat S_{-k}(u|a,X_i)}\left(\frac{\hat S_{0}(u-|a,X_i)}{\hat S_{-k}(u-|a,X_i)}-1\right)(\lambda_0(u|a,X_i) - \hat\lambda_{-k}(u|a,X_i))\right]\Bigg\vert I_k\right]
% \end{align*}
because $K$ is finite and $\hat \lambda_{-k}$ is consistent. Therefore the first term is $o_p(n^{-1/2})$. Finally, the norm of the second term is bounded by:
\begin{align*}
&\norm{\hat S_{-k}(t|a,X_i)\frac{\hat S_{-k}(u-|a,X_i)}{\hat S_{-k}(u|a,X_i)}\left(\frac{S_{0}(u-|a,X_i)}{\hat S_{-k}(u-|a,X_i)}-1\right)(\lambda_0(u|a,X_i) - \hat\lambda_{-k}(u|a,X_i))}_{L_2(P_0)}\\
&\le \norm{\frac{\hat S_{-k}(t|a,X_i)}{\hat S_{-k}(u|a,X_i)}\left(S_{0}(u-|a,X_i) - \hat S_{-k}(u-|a,X_i)\right)(\lambda_0(u|a,X_i) - \hat\lambda_{-k}(u|a,X_i))}_{L_2(P_0)}\\
&\le \norm{\left(S_{0}(u-|a,X_i) - \hat S_{-k}(u-|a,X_i)\right)(\lambda_0(u|a,X_i) - \hat\lambda_{-k}(u|a,X_i))}_{L_2(P_0)}\\
&\le \norm{S_{0}(u-|a,X_i) - \hat S_{-k}(u-|a,X_i)}_{L_2(P_0)}\norm{\lambda_0(u|a,X_i) - \hat\lambda_{-k}(u|a,X_i)}_{L_2(P_0)} = o(n^{-1/2})\\
\end{align*}
since both $\hat \lambda_{-k}$ and $\hat S_{-k}$ have rate $n^{-1/4}$ by assumption \ref{ass:rate_lambda} and lemma \ref{lem:rate_S}. We have shown that each fold $k \in [K]$ and time $u \in \mc T$  is $o_p(n^{-1/2})$. Because $K$ and $|\mc T|$ are finite, we get:
\begin{align*}
\hat \psi(t, a) - \psi_0(t, a) &= P_n[\varphi(t,a,\lambda_0,\omega_0)(O_i)] + \hat \psi(t, a) - P_n[\phi(t, a, \lambda_0, \omega_0)(O_i)]\\
&= P_n[\varphi(t,a,\lambda_0,\omega_0)(O_i)] + \frac{1}{K}\sum_{k=1}^K \sum_{u \le t} (R_{1,u} - R_{2,u} + R_{3,u})\\
&= P_n[\varphi(t,a,\lambda_0,\omega_0)(O_i)] + o(n^{-1/2})
\end{align*}
therefore we have:
\begin{align*}
\sqrt{n}(\hat \psi(t, a) - \psi_0(t, a)) \Longrightarrow \mc N(0, P_0[\varphi(t,a,\lambda_0,\omega_0)(O_i)^2])
\end{align*}
as claimed.
\begin{align*}
\end{align*}
\end{proof}
