# Supplementary material for: A Stable and Efficient Covariate-Balancing Estimator for Causal Survival Effects
Source: arXiv:2310.02278 source file (2024-05-15)
Supplement: Supplementary file 2 [file proof_prop2_2.tex]

\section{Proof of Proposition \ref{prop:identification}}
